# Supplementary material for: Lessons from Deep Learning applied to Scholarly Information Extraction: What Works, What Doesn't, and Future Directions
Source: arXiv:2207.04029 source file (2022-07-08)
Supplement: Supplementary file 1 [file appendixB.tex]

% Github links and general Guideline
\section{Code Delivery and General Guidelines}

We have turned in all the codes through \href{https://github.com/DiscoveryAnalyticsCenter/csetproject}{Github repo}. Please contact pabutler@vt.edu for access issues. We are describing the general outline of the repo below.

\subsection{Directory Structure}
Code for the first five feature extraction tasks are inside \textit{task1} directory. Rests are inside \textit{hardware\_language\_library\_extractor} directory. The repo also contains other tasks under the collaboration of CSET And VT, namely, Dynamic Query Expansion(DQE) and Entity resolution(ER). DQE codes are inside \textit{task2} directory. ER codes are inside \textit{entityResolution} directory. The manually annotated dataset used to evaluate some of the features are inside \textit{evaluation} directory.

\subsection{Data entry point}
The raw data entry point of our repo is \textit{task1/data} directory. It holds input files(pdf,txt) and their structured representation that will be used throughout almost all the pipelines. There are three ways to produce input for our system. You can use PDF, TXT and CSET annotated jsonl files. Directory \textit{data/JSONs/} contains structured representation of the papers that is used as input for our extraction scripts down the line. This is the single data entry point for all extraction subtasks. \\

Each directory and task has a readme file within it. Please contact us or create issues in case anything needs to be addressed.
